# Supplementary material for: Proving Equivalence Between Complex Expressions Using Graph-to-Sequence Neural Models
Source: arXiv:2106.02452 source file (2021-06-09)
Supplement: Supplementary file 1 [file appendix-motivation.tex]

\subsection{Intuitions on Axiomatic Program Equivalence}
\label{subsec:appendix:runningexample}

%%%%%%%%%%%%%%%%%%
\input{figexample1original.tex}
%%%%%%%%%%%%%%%%%%

\paragraph*{Input program representation}

We illustrate in Fig.~\ref{fig:appendix:treeexamples} four very simple computations, represented as graphs, that are all equivalent under various axioms of natural arithmetic.
%% show four examples of simple computations.
For example, \texttt{P1} models the expression $a(1b+1c)$, one can imagine it to be the result of $a(db+dc)$ after e.g. constant-propagation of $1$ to $d$ by a compiler.
They are defined by a single root, have nodes which can be operations consuming the value of their immediate predecessor or terminal/input values, and a node produces a value that can be used by its immediate successors. In essence this is a classical dataflow representation of the computation \cite{buck1993scheduling}, and what our system uses as input program representation.

In this work we represent programs with symbolic expressions made of variables (e.g., $a$, $b$, $c$), operators (e.g., \texttt{+}, \texttt{*}) and neutral/absorbing elements (e.g., $1$). We consider a rich linear algebra expression language, supporting three variable types (scalars as shown in \texttt{P1}-\texttt{P4}, vectors, and matrices) and 5 different variables per type; 16 operators including operators mixing different variable types such as vector-matrix product. Details are provided in Sec.~\ref{sec:appendix:progequivframework} and Sec.~\ref{sec:Axioms}.

\paragraph*{Rewrite rules as axioms of equivalence}
Consider the programs \texttt{P1} versus \texttt{P2}. The multiplication of an integer value by $1$ does not change the value, if we rely on an axiom of equivalence $A1:~ 1_{\mathbb{N}} * x = x,~\forall a \in \mathbb{N}$. This axiom specifies a strict criterion of application: the node must be of type $\mathbb{N}$, the expression pattern must be $1_{\mathbb{N}}*x$; and a strict rewrite rule: replace a sub-graph $1_{\mathbb{N}}*x$ for any $x\in{\mathbb{N}}$ by the graph $x$. In other words, replacing $1*b$ by $b$ in \texttt{P1} is a semantics-preserving rewrite, from the axiom of equivalence $A1$. In this work we view the problem of program equivalence as finding a sequence of semantics-preserving rewrites, each from a precisely defined axiom of equivalence, that rewrites one program into the other. If one program can be rewritten by a sequence of individually-correct semantics-preserving transformations into another one, then not only are they equivalent under the set of axioms used, but the sequence forms the constructive and verifiable proof of equivalence.

\paragraph*{An example} In this work we illustrate and experimentally evaluate our system using a rich linear algebra expression language because it exposes clearly (and intuitively) the various key concepts that must be handled: (1) operating on dataflow graphs as input, supporting transformations that can (2) delete or (3) create new nodes in the graph, and transformations that (4) manipulate entire subtrees. We also wanted a language with (5) multiple variable types, e.g. scalars, vectors and matrices and (6) a large number of different operators with (7) distinct axioms applicable for each. All of these are captured in the language we experiment with, see Sec.~\ref{sec:appendix:progequivframework} for its formal definition.

When applying the axiom $A1:1 * x = x,~\forall x \in \mathbb{N}$ on the program \texttt{P1} for its node $b$, we obtain an equivalent and yet syntactically different program,  we have $P1 \equiv A1(b,P1)$. Applying the same axiom $A1$ on $c$ in the resulting program leads to program \texttt{P2}, and $P2\equiv P1 \equiv A1(c,A1(b,P1))$.
%Precisely, in graph terms, P2 is the result of a sequence of two semantics-preserving node deletion operations, as defined in the axiom.

Consider now the axiom $A2:x * (y+z) = x*y+x*z,~\forall x,y,z \in \mathbb{N}$. This is the standard distributivity axiom on natural arithmetic. In terms of graph transformations, this is a complex rewrite: a new node is created ($*$), one node is moved ($+$ to the root), and edges are significantly modified. When this complex, but semantics-preserving, rewrite is applied to \texttt{P2}, we obtain \texttt{P3}, that is $P3 \equiv A2(*,A1(c,A1(b,P1)))$.

Finally consider the axiom $A3:x+y = y+x,~\forall x,y \in \mathbb{N}$, the standard commutativity axiom for $+$. The graph transformation does not change the number of nodes nor edges, instead only alters two specific edges. Note that as the previous axioms, it also illustrates operations on sub-graphs: indeed $x$ and $y$ do not need to be input/terminal nodes, they can be any subgraph producing a value of the proper type. This is illustrated by applying it on
\texttt{P3} to obtain \texttt{P4}, that is the computation $ac+ab$. We have 
$P4 \equiv A3(+,A2(*,A1(c,A1(b,P1))))$, a verifiable proof of equivalence under our axioms between the programs $a(1b+1c)$ and $ac+ab$, which involved structural changes including node deletion, creation and edge modification. Note the bidirectional nature of the process: one can rewrite from $a(1b+1c)$ to $ac+ab$, or the converse using the same (but reverted) sequence. Note also the non-unicity of a sequence: by possibly many ways a program can be rewritten into another one, for example the sequence $P4 \equiv A3(+,A1(c,A1(b,A2(*,P1))$ also correctly rewrites \texttt{P1} into \texttt{P4}. Conversely, a sequence may not exist: for example no sequence of the 3 above axioms allow to rewrite $a+b$ into $a*b$. We call these non-equivalent in our system, that is precisely if there is no sequence of axioms that can be applied to rewrite one program into the other.

\paragraph*{The need for a verifiable procedure} A key motivation of our work is to enable in a safe and provably correct way the use of machine learning for program equivalence by ensuring no false negative can be produced. For full automation of the process, we focus on ensuring correctness in case an equivalence result is computed by the system. That is, our system by design answers only with a probability of confidence that the two programs are not equivalent, but \emph{it produces a verifiable procedure to assess equivalence} otherwise. We believe such an approach is key for a practical, automated deployment of neural networks for program equivalence: verifiably proving equivalence to ensure no false positive, while tolerating a moderate amount of false negative (i.e., missing that two programs were in fact equivalent).

%Numerous practical applications of the kind of system we develop exist, even on the linear algebra language we demonstrate on: 
Applications of such a system include for example the automatic generation and correction of exercises for students, where they typically need to prove equivalence between two formulas by successive application of other formulas/axioms. Languages like e.g. Matlab could use interactive checking of the equivalence between the expression being typed and the pre-existing library implementations (e.g., BLAS-based \cite{goto2008high}) to use instead accelerated implementations when possible in real-time. But we have designed and evaluated our system in a robust enough way to be applicable to a wide variety of languages and problems, as long as they can be cast in the framework in Sec.~\ref{sec:appendix:progequivframework}.% We discuss other uses cases and applications in Sec.~\ref{sec:expresults}.

\paragraph*{The space of equivalences} Intuitively, our approach to program equivalence is as follows. We can intellectually reason on a graph for equivalent programs where each node represents a distinct program in the language, and two nodes (i.e., two different programs) are connected by a directed edge iff the source node can be rewritten as the target node by the application of a single one of the pre-defined axioms for equivalence. The edge is labeled by the axiom used and the specific position in the source node's program to where it needs to be applied to obtain the program in the target node.
%%%%
Then there will be one or more paths in this graph from the two nodes modeling the two input programs if they are equivalent (one can be rewritten into the other while preserving semantics); and no path if no such rewrite is possible, that is the programs would be not equivalent in our framework. Exposing a path between two nodes is sufficient to prove the equivalence of their associated programs.

This path is exactly a sequence of rewrite rules from one program to another. To test the correctness of an arbitrary sequence, i.e., verify if this path exists in the graph and assess equivalence if it does, one then needs to simply apply the proposed sequence to one of the input programs: verify at each step that the rewrite in the sequence is indeed applicable (by a simple check of the applicability of the axiom at this particular program point), and eventually ensure the rewritten program is identical to the other input one. This test can be computed in time mostly linear with the program size in our framework, and when successful it implements a constructive proof of equivalence between the two programs.

\paragraph*{Pathfinding equivalence proofs}
When formulating the program equivalence problem this way, we can then view its solution as learning how to build at least one feasible path between any two pairs of nodes in the above graph, when it can exist. We can see that by design, there is a lot of redundancy in this space: the same labeled path will occur between many different pairs of programs (e.g., those where only the variable symbols differ), and there are typically many paths between the same two (equivalent) programs. This creates opportunities for the system to learn program representation and path construction techniques more easily.

Our key contribution is the development of a deep learning framework that learns this procedure automatically. The neural network system we build is trained by randomly sampling this graph, with samples made of two nodes and a path between them when training on equivalent programs, and an empty path otherwise. We specifically learn a generalization of the problem of finding paths in this graph as follows. We represent input programs in a carefully-crafted normalized dataflow-like graph encoded as a gated graph neural network \cite{Scarselli09,Beck18}, to enable structural, size-tolerant reasoning by the network on the inputs. It is combined with a global attention-based mechanism and a memory-based LSTM \cite{Hochreiter97} decoder which can memorize graph changes for producing the rewrite sequence and enable path-size tolerant reasoning, while following the properties of the axioms for equivalence.

In a nutshell, we make the network learn a stochastic approximation of an iterative algorithm that would be able to construct a feasible path (when possible) between any two pairs of nodes in this equivalence graph, but trained simply by randomly sampling pairs of nodes and one carefully labeled path between them. This avoids entirely the need to craft smart exploration heuristics to make this path-finding problem feasible in practice. This is instead what we let the neural network learn automatically; and specifically why we implemented graph neural networks to solve this problem \cite{Scarselli09,Xu17}. We rely on the network to suggest a transformation path by inference, and then verify its validity in linear time.

\subsection{System Overview}
\label{subsec:appendix:systemoverview}

\begin{figure*}
\includegraphics[width=14cm]{./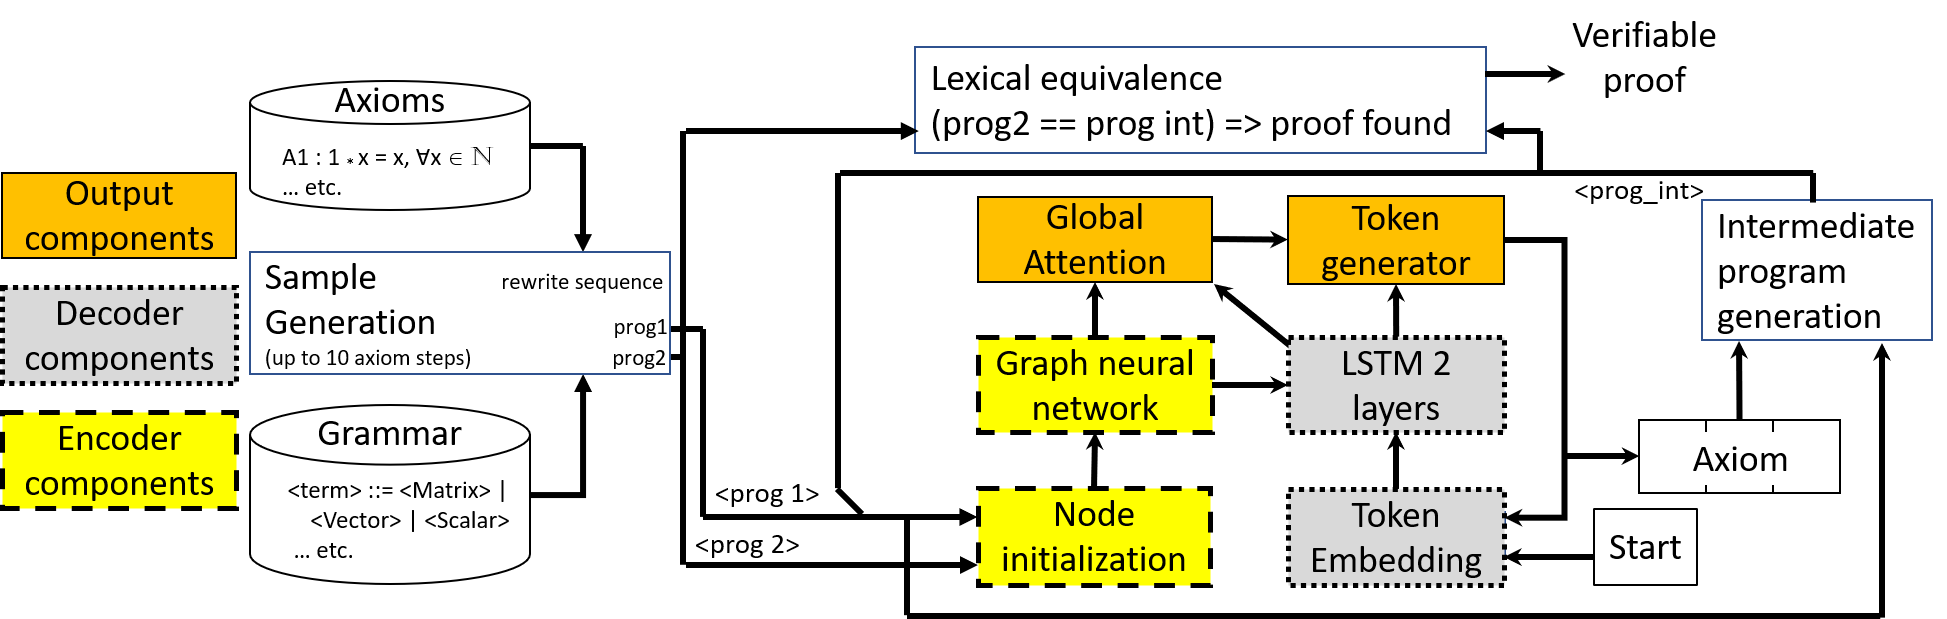}
\caption{\texttt{pe-graph2axiom} System Overview}
\label{fig:Full:appendix}
\end{figure*}

To implement our approach, we enumerate randomly valid sentences in a language, and a set of axioms of equivalence expressible as semantics-preserving rewrite rules from one to the other. 
The system in Fig.~\ref{fig:Full:appendix} takes as input two programs represented as symbolic trees representing a dataflow graph of an expression computation, and eventually produces a sequence of axioms along with their position of application (or node) that can be used to rewrite sequentially one input program into the other input program. 
As each axiom is produced, it is checked to insure it is a legal application within the grammar and if the transformed program matches the target then a correct proof of equivalence has been found.
To train the system, we generate pairs of equivalent programs by iterating the axioms with random probability on one program, thereby generating both a path to equivalence and the target program. Random programs are generated so as to respect the grammar defined. The training set is then appropriately selected from these random samples, as detailed in Sec.~\ref{sec:suppl:neuralnetwork}.
%The system in Fig.~\ref{fig:Full}  is composed of the following blocks. 
\emph{Node initialization} initializes the graph neural network, converting the input programs text (e.g., $(a+(b+c))$ into nodes and edges in the \emph{Graph Neural Network} \cite{Scarselli09,Xu17}.
%refers to a neural network that has weights which allow it to learn interrelations between network nodes based on edge connections.
%We use \emph{Global attention} \cite{luong15} to connect tokens produced with nodes in the graph.
%allows the decoder to pay attention to certain nodes in the graph as it creates each token in the output sequence.
%
%A key of our approach is to introduce graph-to-sequence neural networks to quickly compute one or more possible rewrite sequences. 
%
The details of the network are covered in Sec.~\ref{sec:progequivdnn}. In a nutshell, the key principle is to combine a memory-based neural network approach, e.g., using Long-Short Term Memory (LSTM) \cite{Hochreiter97} neurons and a graph neural network design (which uses Gated Recurrent Units (GRUs) internally) \cite{Beck18} that matches our program graph representation.  \emph{Token embedding} is a neural network layer in which tokens are assigned a learnable multidimensional embedding vector \cite{Mikolov13}.
Each layer in \emph{LSTM 2 layers} has 256 neurons, which support sequence generation.
\emph{Token generator} is the final output portion of the network. It learns to output the tokens based on the current LSTM hidden states and the \emph{Global Attention} from the graph neural network. As each token is output, it feeds back into the LSTM layer through the embedding layer to affect its next state. We use a sequence 
generation principle, using a global attention mechanism \cite{luong15} to allow observation of program graph node information while generating the axiom and location on which it is applied. As developed below, we specifically study the robustness of our approach to generate proofs of increasingly complex length, contrasting models to output the entire path at once with \texttt{pe-graph2axiom} which incrementally builds the sequence one step at a time, as shown in Sec.~\ref{sec:suppl:additionalresults}.
